# Supplementary material for: Calorimeters for the FCC-hh
Source: arXiv:1912.09962 source file (2019-12-20)
Supplement: Supplementary file 1 [file appendix.tex]

%This is the appendix
